# Supplementary material for: StagedWorkspace: A Versioned Workspace for Knowledge-Work Agents
Source: arXiv:2608.18050 source file (2026-08-18)
Supplement: Supplementary file 1 [file appendix_agent_inference.tex]

\subsection{Agent inference configuration}
\label{app:agent-inference}

\paragraph{Tool-call budget.}
All benchmark runs share a 250-tool-call budget per agent attempt (Section~\ref{sec:setup-benchmarks}), matching the \textsc{APEX-Agents} step limit~\citep{apexagents2026}.
The harness counts each assistant tool-call round toward this budget; the agent may submit a final answer or deliverable before exhaustion.

\paragraph{Per-model decoding.}
Table~\ref{tab:agent-model-configs} lists the hosted model IDs, reasoning levels, and decoding settings used for \emph{agent} inference in our ablations.
Reasoning levels follow the public benchmark tables for matched models (Section~\ref{sec:setup-benchmarks}); we do not restate the main-text model roster here.
We do not set an explicit sampling temperature in the harness: OpenAI reasoning models use the provider default (no temperature parameter); Gemini models use the provider default of $1.0$; Kimi K2.6 uses temperature $0.7$ as in~\citet{apexagents2026}.
Maximum \emph{output} tokens per agent turn is 64{,}000 (engine default); there is no separate input-token cap beyond each model's published context window.

\begin{table}[t]
  \centering
  \caption{Agent inference settings by model (ablation runs). Input limits are each model's published context window; output cap is 64{,}000 tokens for all rows.}
  \label{tab:agent-model-configs}
  \small
  \setlength{\tabcolsep}{4pt}
  \begin{tabular}{@{}llllr@{}}
    \toprule
    Benchmark & Model & Reasoning & Temp. & Max out. \\
    \midrule
    OfficeQA & \texttt{openai/gpt-5.4} & High & --- & 64k \\
    OfficeQA & \texttt{google/gemini-3.1-pro-preview} & High & 1.0 & 64k \\
    OfficeQA & \texttt{google/gemini-3-flash-preview} & High & 1.0 & 64k \\
    \midrule
    \textsc{APEX} & \texttt{openai/gpt-5.4} & xHigh & --- & 64k \\
    \textsc{APEX} & \texttt{openai/gpt-5.4-mini} & xHigh & --- & 64k \\
    \textsc{APEX} & \texttt{openai/gpt-5.4-nano} & xHigh & --- & 64k \\
    \textsc{APEX} & \texttt{google/gemini-3-flash-preview} & High & 1.0 & 64k \\
    \textsc{APEX} & \texttt{google/gemini-3.1-pro-preview} & High & 1.0 & 64k \\
    \textsc{APEX} & \texttt{moonshot/kimi-k2.6} & default & 0.7 & 64k \\
    \bottomrule
  \end{tabular}
\end{table}

\paragraph{Context management and compaction.}
When estimated session input tokens reach 65\% of the resolved model context window, the harness triggers compaction mid-turn (inside the tool loop) or post-turn (stop hook).
OpenAI and Azure routes use provider-native \texttt{/responses/compact} when supported; Gemini and other providers summarize prior context via a \texttt{write\_memory} tool call.
Compaction history loading uses the same 65\% budget fraction.
Tool outputs longer than ${\approx}10$\,k tokens are truncated before returning observations to the agent.
Unlike the \textsc{OfficeQA Pro} custom agent's fixed 30-message sliding window~\citep{officeqa2026}, our harness compacts on token fill rather than a message count.

\paragraph{Grading models (fixed across ablations).}
Grader sessions are separate from agent inference; model and decoding settings are fixed per benchmark and identical across artifact-access arms (Appendix~\ref{app:grader-protocols}).
\textsc{OfficeQA Pro} uses deterministic exact-match semantics aligned with the public \texttt{reward.py} convention (0.0\% allowable absolute relative error)~\citep{officeqa2026}.
\textsc{APEX-Agents} uses \texttt{google/gemini-3-flash-preview} with thinking level \emph{low}, matching the public benchmark grader~\citep{apexagents2026}.
